# Supplementary material for: Dark Matter Detection Using Helium Evaporation and Field Ionization
Source: arXiv:1706.00117 ancillary file (2017-09-22)
Supplement: Supplementary file 1 [file supplemental-material-DM-detection.pdf]

# Supplemental Material: Dark Matter Detection Using Helium Evaporation and Field Ionization

Humphrey J. Maris,[1] George M. Seidel,[1] and Derek Stein[1]
[1]*Department of Physics, Brown University, Providence, Rhode Island 02912, USA*

## POSSIBLE ADVERSE EFFECTS

The measurement of single evaporated helium atoms using field ionization presents a number of interesting technical problems regarding the suppression of noise introduced by the detector itself. The field ionization detector, consisting of an array of sharp tips forming the anode and a planar cathode operating possibly at a potential difference of as much as 50 MV/m, functions by ionizing helium atoms at the sharp tips followed by the their subsequent acceleration to the cathode where their energy deposition can be measured calorimetrically. This process carries with it several potential collateral effects that could detrimentally influence the measurements if not properly accounted for. These effects are discussed here.

### Sputtering

A helium ion striking the cathode with a few keV of energy can sputter atoms from the cathode surface. A sputtered atom can return to the high field tip, become ionized, and be accelerated back to the cathode leading to further sputtering. Helium being a light atom has a low probability of sputtering. If the cathode is coated by a low-atomic-number metal like beryllium, the sputtered atom also is light and on returning to the cathode produces minimal additional sputtering. For a 50 keV helium ion hitting beryllium, the probability of sputtering is only 1 % [1], and the probability of beryllium self-sputtering at 50 keV is about 10 % [2]. Therefore, if beryllium were the cathode material sputtering would not be a concern.

Other materials might also be suitable for coating the cathode in order to eliminate the possibility of a runaway self-sputtering process. The crucial requirement is that the self-sputtering yield of that material be less than one. It is worth pointing out that the material used to coat the cathode surface could be a compound composed of multiple elements and it need not be a metal. For a titanium cathode, a metal that is known to be capable of having very low field emission at 50 keV (see section on field emission below), the situation for sputtering is less favorable. The probability that a helium ion at 50 keV will sputter titanium is only 1 % [1], but a sputtered titanium atom, ionized at the anode, is likely to produce two sputtered atoms upon returning to the cathode. However, oxidizing the surface of a titanium cathode might reduce the sputter yield sufficiently to solve the problem.

Because the signal produced by sputtered atoms occurs essentially coincident with the initiating event, this process does not lead to dark counts, although it does result in a misidentification of the number of ionized helium atoms. This uncertainty in identifying the number of helium atoms ionized in a specific event is inconsequential given the broad probability distribution of the number of evaporated atoms produced by a recoil event of given energy in the target and the probability that evaporated atoms will be ionized.

### Secondary electron emission

Helium atoms can also produce secondary electrons upon hitting the cathode. An average of about 1.5 secondary electrons are produced by a 50 keV helium ion when striking a light metal [3]. These electrons will be accelerated back to hit the anode thereby generating X-rays. However, the process of X-rays generation by electron impact is notoriously inefficient both for characteristic lines and for bremsstrahlung. In an X-ray tube roughly only 1 % of the electron kinetic ends up as photons. Given the design of the detector, the X-rays are most likely to travel in a direction so as to hit the cathode. Since the cathode serves as the calorimeter for detecting the $He^+$ ions, it must have low heat capacity and thus be relatively thin ($\sim 1\ \mu$m). As a consequence an X-ray has a low probability of depositing energy in the cathode. A 50 keV X-ray loses energy principally by Compton scattering, the maximum energy loss for such an X-ray being 15 keV. While some fraction of the energy of an X-ray will be deposited in the components of the ionization detector, much of it will end up in the walls of the cryostat.

X-rays may also, with low probability, enter the material serving as the target for dark matter particle interactions. If the target is liquid helium, the consequences of a 50 keV X-ray Compton scattered in the liquid would be to produce additional helium evaporation, but time delayed by more than 0.1 ms from the triggering event because of the low velocity of rotons. The time constant of the calorimeter/cathode should easily have the ability to identify such correlated signals. In the case that the target material is a crystal the time delay will be about a factor of 10 shorter, but the enhanced ability of

event location provides another handle for discrimination between a Compton scatter and the triggering energy deposition.

### Electron field emission from the cathode

It is well known that a planar cathode subject to an electric field can emit electrons at fields much lower than predicted by Fowler-Nordheim theory [4] due to the existence of small protuberances on the surface where the field can be enhanced by orders of magnitude over that on the flat surface. The field enhancement has not been reduced below value of several hundred on stainless steel [5] and copper cathodes [6] in spite of serious efforts involving a variety of polishing, gas conditioning and coatings to improve their performance [7]. Such enhancements result in dark currents of nanoamperes per square centimeter at a field of 50 MV/m.

On the other hand, cathodes of niobium [8], titanium and molybdenum [9] have been fabricated having field enhancements of a few tens and can be operated up to applied fields of 80 MV/m without a measurable dark current. We base the following discussion of noise on the use of titanium as the cathode.

The Fowler-Nordheim equation [4] for the current density, $j$, in $\mathrm{A\,nm^{-2}}$ is

$$j = \frac{aE^2}{\phi} \exp\left(-\frac{g(f) b \phi^{3/2}}{E}\right), \quad (1)$$

where the constants are $a = 1.54 \times 10^{-6}$ A eV V$^{-2}$ and $b = 6.83$ eV$^{-3/2}$ V nm$^{-1}$. $\phi$ is the work function of the metal in eV, $E$ is the electric field in $\mathrm{V\,nm^{-1}}$, while the dimensionless parameter $g(f) = 1 - f + \frac{1}{6}\ln f$, with $f = (1.44\ \mathrm{eV^2V^{-1}\ nm})(E/\phi^2)$. The quantity $E$ is the field enhanced at the protuberance, $E = \gamma E_m$, $E_m$ being the applied macroscopic field and $\gamma$ the enhancement factor. For a metal with a work function $\phi = 4.4$ eV and an enhancement factor of $\gamma = 27$ [9] the calculated dark current is an extremely sensitive function of the applied field in the vicinity of 0.05 V nm$^{-1}$. Small changes in the parameters can lead to estimates varying from $10^{-4}$ to $10^4$ electron emissions per second for a protuberance with area of $10^{-15}$ nm$^2$. Careful attention must be paid to the surface quality of the cathode to ensure a low emission rate (well below 1 s$^{-1}$), the rate of secondary electron emission induced by impact of $He^+$ ions, discussed above. Surface layers such as oxides and nitrides can have a beneficial effect in that they tend to increase the work function and lower electron emission.

Finally, the design of the proposed field ionization detector, which calls for a silicon wafer to be used as a calorimeter in contact with the cathode, opens up the possibility of obtaining extraordinarily flat cathode surfaces made of virtually any material. This is because it is relatively straightforward to deposit tens of nanometers of an arbitrary metal on the near-atomically flat surface of a polished silicon wafer without creating significant protuberances. Thus it should be possible to fabricate a beryllium cathode that exhibits both low self-sputtering yield and a sufficiently low electron field emission rate.

### Helium migration

In addition to the usual dark counts generated by background radiation, the field ionization detector has the several potential additional sources of noise. Any helium atoms adsorbed in the vicinity of the high field tip may diffuse to the tip with the aid of the polarization force and be interpreted falsely as originating from evaporation. It is expected that this source of dark counts can be reduced to an inconsequential rate by heating the ionization detector to a high temperature, such as 20 K for several minutes prior to operation, with the helium liquid remaining at 20 mK and the film burner operating so as to keep any new atoms from migrating to the heated surface. The helium atoms desorbed from the detector will condense on the unheated film-covered surfaces or the free surface of the liquid. This is a procedure used in the HERON experiment to clear the calorimeters of adsorbed helium [10].

### Field evaporation

If the field at the tips becomes high, atoms composing the tip can become detached, ionized and travel to the cathode, a process called field evaporation. Tungsten ions can detach from the tip surface when the local electric field exceeds 6 V/Å. This process has been used to condition tips; by raising the tip potential above the value desired for operation, the surface atoms that form asperities, and hence the highest local field, are removed, leaving a tip with a larger and more uniform radius. The field for evaporation of tip materials selected for field ionization of gas atoms must be higher than that for ionization, and by operating the detector at the proper potential this process is not expected to be an issue.

---

[1] N. Matsunami, Y. Yamamura, Y. Itikawa, N. Itoh, Y. Kazumata, S. Miyagawa, K. Morita, R. Shimizu, and H. Tawara, Atomic data and nuclear data tables **31**, 1 (1984).

[2] M. Guseva, V. Gureev, S. Korshunov, V. Neumoin, Y. A. Sokolov, V. Stolyarova, V. Vasiliev, S. Rylov, and V. Strunnikov, Journal of nuclear materials **220**, 957 (1995).

[3] R. Ramachandra, *A study of helium ion induced secondary electron production*, Ph.D. thesis, University of Tennessee Knoxville (2009).

[4] R. G. Forbes and J. H. Deane, in *Proceedings of the Royal Society of London A: Mathematical, Physical and Engineering Sciences*, Vol. 463 (The Royal Society, 2007) pp. 2907–2927.

[5] M. BastaniNejad, A. A. Elmustafa, E. Forman, S. Covert, J. Hansknecht, C. Hernandez-Garcia, M. Poelker, L. Das, M. Kelley, and P. Williams, Journal of Vacuum Science & Technology A: Vacuum, Surfaces, and Films **33**, 041401 (2015).

[6] C. Suzuki, T. Nakanishi, S. Okumi, T. Gotou, K. Togawa, F. Furuta, K. Wada, T. Nishitani, M. Yamamoto, J. Watanabe, *et al.*, Nuclear Instruments and Methods in Physics Research Section A: Accelerators, Spectrometers, Detectors and Associated Equipment **462**, 337 (2001).

[7] M. Bastaninejad, A. Elmustafa, E. Forman, J. Clark, S. Covert, J. Grames, J. Hansknecht, C. Hernandez-Garcia, M. Poelker, and R. Suleiman, Nuclear Instruments and Methods in Physics Research Section A: Accelerators, Spectrometers, Detectors and Associated Equipment **762**, 135 (2014).

[8] A. D. Pandey, G. Müller, D. Reschke, and X. Singer, Physical Review Special Topics-Accelerators and Beams **12**, 023501 (2009).

[9] F. Furuta, T. Nakanishi, S. Okumi, T. Gotou, M. Yamamoto, M. Miyamoto, M. Kuwahara, N. Yamamoto, K. Naniwa, K. Yasui, *et al.*, Nuclear Instruments and Methods in Physics Research Section A: Accelerators, Spectrometers, Detectors and Associated Equipment **538**, 33 (2005).

[10] R. Torii, S. Bandler, T. More, F. Porter, R. Lanou, H. Maris, and G. M. Seidel, Review of scientific instruments **63**, 230 (1992).
